# Supplementary material for: Quantum-Limited Squeezed Light Detection with a Camera
Source: arXiv:2006.10573 ancillary file (2020-06-18)
Supplement: Supplementary file 1 [file Squeezed_Light_Detection_Using_Quantum_Imaging_supp.pdf]

# Supplementary Material: "Quantum-Limited Squeezed Light Detection with a Camera"

Elisha S. Matekole,[1] Savannah L. Cuozzo,[2] Nikunjkumar Prajapati,[2] Narayan Bhusal,[1] Hwang Lee,[1] Irina Novikova,[2] Eugeniy E. Mikhailov,[2] Jonathan P. Dowling,[1,3,4,5] and Lior Cohen[1,6]

[1]*Hearne Institute for Theoretical Physics, and Department of Physics and Astronomy, Louisiana State University, Baton Rouge, Louisiana 70803, USA.*

[2]*Department of Physics, William and Mary, Williamsburg, VA 23187, USA*

[3]*NYU-ECNU Institute of Physics at NYU Shanghai, 3663 Zhongshan Road North, Shanghai, 200062, China.*

[4]*CAS-Alibaba Quantum Computing Laboratory, CAS Center for Excellence in Quantum Information and Quantum Physics, University of Science and Technology of China, Shanghai 201315, China.*

[5]*National Institute of Information and Communications Technology, 4-2-1, Nukui-Kitamachi, Koganei, Tokyo 184-8795, Japan*

[6]*cohen1@lsu.edu*

(Dated: June 17, 2020)

In here, we describe the simulation of the beam propagation and the camera operation. To keep the discussion as general as possible, we generalize the single-mode theory of the main text to a multi-mode theory. We, first, propagate the multi-mode beam through the medium. Then, we simulate the finite-sampling experiment by randomly choosing photon numbers distributed as the theoretical photon statistics. In addition, an example of turbulence is given, and the extraction method of the squeezing parameter is demonstrated.

PACS numbers: Valid PACS appear here

### Multimode state propagation

We assume the incoming light has a Gaussian shape profile and its photon number distributed as displaced squeezed vacuum state. Mathematically the state is a product state; $|\Psi\rangle = |\psi\rangle_{0,0}|0\rangle_{1,0}...|0\rangle_{h,g}...$ where $|\phi\rangle_{h,g}$ is a state, $|\phi\rangle$, in the h,g Hermite-Gaussian mode [1] and $|\psi\rangle_{0,0} = \hat{D}(\alpha)\hat{S}(\xi)|0\rangle_{0,0}$ is the displaced squeezed vacuum state in the Gaussian mode. Any state can be written with Fock expansion:

$$|\psi\rangle_{0,0} = \sum_{n=0}^{\infty} c_n (a^\dagger_{0,0})^n |0\rangle \,. \tag{S1}$$

Due to the medium the state scatters from the Gaussian mode to other Hermite-Gaussian modes. In general, the amplitude can scatter to unaccessible modes, which introduces loss to the system. In this scenario, our method still works as we do not require controllable or known loss to apply it. The scattering matrix, $B_{h,h',g,g'}$, is found by integrating over the product of the eigenfunctions before and after the medium [2]. Because the initial state is a single-mode, the amplitude of the $h'$, $g'$ mode is $B_{0,h',0,g'}$. Similarly, after quantization, we get: $a^\dagger_{h',g'} = B^*_{0,h',0,g'} a^\dagger_{0,0}$, where $B^*$ stands for the conjugate (without transpose) of $B$. Inverting the last relation we get: $a^\dagger_{0,0} = \sum_{h',g'} b(h',g') a^\dagger_{h',g'}$, where $b_{h',g'}$ are the coefficients of the inverse matrix of $B^*_{h,h',g,g'}$, after substituting $h = 0, g = 0$. Substituting $a^\dagger_{0,0}$ in Eq. S1 we get:

$$|\Psi\rangle = \sum_{n=0}^{\infty} c_n \Big( \sum_{h',g'} b_{h',g'} a^\dagger_{h',g'} \Big)^n |0, ..., 0, ...\rangle \,, \tag{S2}$$

which is the state after the medium.

Now we want to return to the camera (position) basis. Thus, we apply another transformation; $a^\dagger_{h',g'} = \sum_{x,y} U_{h',g'}(x,y) a^\dagger_{x,y}$, where $U_{h',g'}(x,y)$ is the eigenfunction of the $h', g'$ Hermite-Gaussian mode. Substituting $a^\dagger_{h',g'}$ in Eq. S2, the final state upon the camera is revealed:

$$|\Psi\rangle = \sum_{n=0}^{\infty} c_n \Big( \sum_{h',g'} b_{h',g'} \sum_{x,y} U_{h',g'}(x,y) a^\dagger_{x,y} \Big)^n |0, ..., 0, ...\rangle \,. \tag{S3}$$

Because no correlation measurements are used, we can focus on one pixel $x', y'$;

$$|\Psi\rangle = \sum_{n=0}^{\infty} c_n \sum_{k=0}^{n} \binom{n}{k} \Big( \sum_{h',g'} b_{h',g'} U_{h',g'}(x',y') a^\dagger_{x',y'} \Big)^k \Big( \sum_{x\neq x', y\neq y'} \sum_{h',g'} b_{h',g'} U_{h',g'}(x,y) a^\dagger_{x,y} \Big)^{n-k} |0, ..., 0, ...\rangle \,, \tag{S4}$$

where we switch the summation order and exclude the $x', y'$ pixel from the sum. One can see immediately from Eq. S4 that the photon statistics of the $x', y'$ pixel are

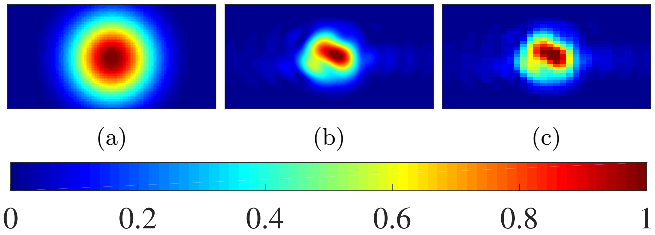


FIG. S1: (ColorOnline). Beam profile before (a) and after (b-c) the exampled medium. (c) shows the field amplitudes after binning to 32-by-32 camera pixels.

identical to the displaced-squeezed-vacuum statistics after loss of $1 - |\sum_{h',g'} b_{h',g'} U_{h',g'}(x',y')|^2$ (1- efficiency, where efficiency is the fraction of field amplitude, incident the other pixels). Without the medium the summation will be gone and only the Gaussian profile, $|U_{0,0}(x',y')|^2$, will remain. Unsurprisingly, this confirms our camera model with an adjustable loss operation, the exact same operation as we got from the multi-mode model. Figure S1 shows the field amplitudes before and after the scattering for an example of a diffusive medium [3].

### Simulation procedure and raw results

Next, we simulate a shot of the camera. First, we choose randomly a photon number according to the statistics of the displaced-squeezed-state [4], and then, the photons are randomly distributed among the 32-by-32 camera pixels, according to the amplitudes of Fig. S1c. After repeating the random process N times, the intensity and variance are computed for each pixel individually.

Since each pixel has a different collection efficiency value, plotting its variance as a y-value and its intensity as an x-value gives a parametric plot of the efficiency parameter. Figure S2 shows this parametric plot for N=100 and N=10,000 camera shots, where the pixel's efficiency values were taken from Fig. S1c and the physical values are $\bar{n}_s = 1$, and $\bar{n}_\alpha = 10^6$.

As a side note, here, we focus on the camera framework thus we use 'efficiency' as the description of the partial field incident on one pixel. However, in the main text we focus on the tunable attenuator, thus we use 'transmission' to describe the same parameter.

According to the theory of the main text, if we fit the variance to a quadratic polynomial, the squeezing parameter is extracted from the quadratic coefficient. Thus, we should examine the precision of this coefficient. For the $N = 100$ case, the quadratic coefficient is $-3.1 \times 10^{-6} \pm 0.7 \times 10^{-6}$ and $2.1 \times 10^{-6} \pm 0.6 \times 10^{-6}$ for squeezed (Fig. S2a) and anti-squeezed (Fig. S2b) states. Similarly for the $N = 10,000$ case, the quadratic coefficient is $-7.3 \times 10^{-7} \pm 0.8 \times 10^{-7}$, and $4.95 \times 10^{-6} \pm 0.07 \times 10^{-6}$ for squeezed (Fig. S2c) and anti-squeezed (Fig. S2d) states respectively. Theoretically, the quadratic coefficient is $-8.284 \times 10^{-7}$ and $4.828 \times 10^{-6}$ for squeezed and anti-squeezed state respectively (see Eq. 3 of the main text).

While the precision is tremendously improved when the number of iterations is increased, there is still a gap between the theory and simulations. This gap is a consequence of the large number of pixels: More pixels means smaller efficiency of each pixel. Therefore the efficiency is typically limited to 1% and we do not get enough range of efficiency. By summing over pixels, we can increase the efficiency range and substantially increase the precision of the extracted coefficient. This part is shown and discussed in the main text.

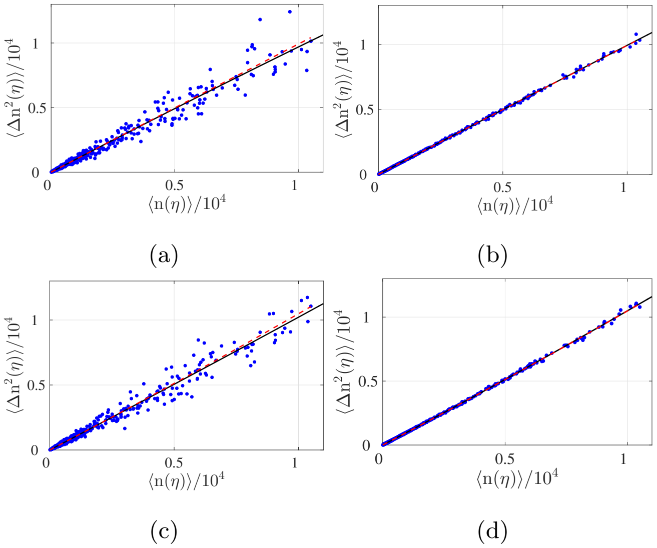


FIG. S2: (ColorOnline) The simulation results of the variance as a function of the intensity for 100 **(a)** and **(d)** and 10,000 iterations with squeezed **(a-b)** and **(c-d)** anti-squeezed states. Every data point represents a different pixel. In all sub-figures the state parameters are; $\bar{n}_\alpha = 10^6$ and $\bar{n}_s = 1$. The solid black line is a fit to second order polynomial, and the dashed red line is the theoretical relation, obtained from Eq. 2 in the main text.

[1] A. E. Siegman, *Lasers* (University Science Books, 1986).
[2] Z. Xiao, R. N. Lanning, M. Zhang, I. Novikova, E. E. Mikhailov, and J. P. Dowling, Phys. Rev. A **96**, 023829 (2017).
[3] J. P. Bos, M. C. Roggemann, and V. R. Gudimetla, Appl. Opt. **54**, 2039 (2015).
[4] C. Gerry and P. Knight, *Introductory Quantum Optics* (Cambridge University Press, Cambridge, UK, 2005).
